# Supplementary material for: FCGHunter: Towards Evaluating Robustness of Graph-Based Android Malware Detection
Source: arXiv:2504.19456 source file (2025-04-28)
Supplement: Supplementary file 1 [file 10-appendix.tex]

% \section{appendix}

\subsection{Detailed Introduction about Graph Embeddings}
\subsubsection{\malscan}\label{detailed_malscan}
\hfill \\
\textbf{Degree Centrality} measures a node's direct connectivity by tallying its direct links, providing a simple gauge of its involvement in the graph. In a directed FCG, the degree feature for a node $v$ is the sum of its in-degree and out-degree.
\begin{equation}
    \footnotesize
    C_D(v) = \frac{\text{degree}(v)}{N-1}
\end{equation}
where $degree(v)$ represents the number of edges connected to node $v$, and $N$ is the number of nodes in the FCG.

\noindent\textbf{Katz Centrality} evaluates a node's influence by summing the weighted paths that reach it, where the weight of each path diminishes exponentially with its length. This centrality metric captures both the local and extended influence of a node.
\begin{equation}
    \footnotesize
    C_K(v) = \sum_{k=1}^{\infty} \sum_{i=1}^{N} \alpha^k \cdot (A^k)_{iv}
\end{equation}
where $k$ represents the path length, $i$ is an indexing variable that sums over all nodes, $\alpha$ is a constant attenuation factor less than the reciprocal of the largest eigenvalue of $A$ that reduces the contribution of longer paths, and $(A^k)_{iv}$ is the $i,v$-th entry of the $k$-th power of the adjacency matrix $A$, representing the number of paths of length $k$ from node $i$ to node $v$.

\noindent\textbf{Harmonic Centrality} incorporates the harmonic mean in calculating nodal centrality, highlighting the significance of nodes bridging distant network sections. It assigns inverse weights to the shortest paths to all nodes, ensuring even the furthest nodes influence the centrality score.
\begin{equation}
    \footnotesize
    C_H(v) = \sum_{u \neq v} \frac{1}{d(u,v)}
\end{equation}
where $d(v,u)$ means the shortest path distance between node $u$ and $v$.

\noindent\textbf{Closeness Centrality} measures the average length of the shortest paths from a node to all others in the network, thus depicting the node's propensity to access or disseminate information swiftly.
\begin{equation}
    \footnotesize
    C_C(v) = \frac{(N_r-1)^2}{\sum_{u=1}^{N-1} d(u,v) \times (N-1)}
\end{equation}
where $N_r$ is the number of reachable nodes from node $v$, and the $ \frac{(N_r-1)^2} {(N-1)}$ ensures normalization by the size of the reachable network. 
% This is different from the calculation in other fields~\cite{zhang2017degree}.

\noindent\textbf{Average} (i.e., equation \ref{eq:average_centrality}) and \textbf{Concentrate} (i.e., equation~\ref{eq:concentrate_centrality}) centralities combine the four above metrics in comprehensive features.
\begin{equation}
    \footnotesize
    C_{AVG}(v) = \frac{C_D(v) + C_K(v) + C_H(v) + C_C(v)} {4}
    \label{eq:average_centrality}
\end{equation}
\vspace{-0.15cm}
\begin{equation}
    \footnotesize
    C_{CON}(v) = concentrate(C_D(v), C_K(v), C_H(v), C_C(v))
    \label{eq:concentrate_centrality}
\end{equation}

\subsubsection{\mamadroid}\label{detailed_mamadroid}
\hfill\\
%mamadroid的特征是一个矩阵，里面的每一个值代表转移的概率。
The features of \mamadroid are represented as a matrix, where each value denotes the probability of transition.
The probability \( P_{jk} \) of transitioning from one API call \( j \) to another API call \( k \) in the Markov chain can be expressed as:

\begin{equation}
    \footnotesize
    P_{jk} = \frac{O_{jk}}{\sum_{i \in S} O_{ji}}
\end{equation}
where \( O_{jk} \) is the observed count of how often API call \( j \) is immediately followed by API call \( k \). The denominator is the sum of counts of all observed transitions from API call \( j \) to any API call within the set \( S \), which is the set of all possible states (or API calls) that can follow \( j \). This normalizes \( O_{jk} \) to a probability distribution over all possible subsequent API calls.

\begin{table*}[!t]
\centering
\caption{Detection performance of the ML-based AMD
methods.}
\label{tab:model_eval}
\resizebox{.99\textwidth}{!}{
\begin{tabular}{c|ccccc|ccccc|ccccc|ccccc}
\hline
                   & \multicolumn{5}{c|}{MalScan (Degree)}  & \multicolumn{5}{c|}{MalScan (Katz)}        & \multicolumn{5}{c|}{MalScan (Harmonic)} & \multicolumn{5}{c}{MalScan (Closeness)} \\ \cline{2-21} 
\multirow{-2}{*}{} & MLP    & KNN-1  & KNN-3  & RF   & AB   & MLP     & KNN-1   & KNN-3  & RF    & AB    & MLP   & KNN-1  & KNN-3  & RF    & AB    & MLP   & KNN-1  & KNN-3  & RF    & AB    \\ \hline
\rowcolor[HTML]{CFE2F3} 
Accuracy           & 0.94   & 0.93   & 0.93   & 0.92 & 0.91 & 0.95    & 0.93    & 0.93   & 0.92  & 0.91  & 0.95  & 0.81   & 0.93   & 0.91  & 0.90  & 0.95  & 0.93   & 0.93   & 0.92  & 0.91  \\
Precision          & 0.98   & 0.95   & 0.97   & 0.92 & 0.91 & 0.96    & 0.96    & 0.96   & 0.92  & 0.93  & 0.95  & 0.95   & 0.96   & 0.90  & 0.86  & 0.98  & 0.95   & 0.95   & 0.93  & 0.87  \\
\rowcolor[HTML]{CFE2F3} 
Recall             & 0.91   & 0.91   & 0.91   & 0.92 & 0.91 & 0.94    & 0.92    & 0.92   & 0.92  & 0.89  & 0.95  & 0.74   & 0.91   & 0.93  & 0.94  & 0.92  & 0.91   & 0.92   & 0.92  & 0.94  \\
F1                 & 0.94   & 0.93   & 0.94   & 0.92 & 0.91 & 0.95    & 0.94    & 0.94   & 0.92  & 0.91  & 0.95  & 0.83   & 0.93   & 0.91  & 0.90  & 0.95  & 0.93   & 0.93   & 0.92  & 0.90  \\ \hline \hline
                   & \multicolumn{5}{c|}{MalScan (Average)} & \multicolumn{5}{c|}{MalScan (Concentrate)} & \multicolumn{5}{c|}{Mamadroid}          & \multicolumn{5}{c}{APIGraph}            \\ \cline{2-21} 
\multirow{-2}{*}{} & MLP    & KNN-1  & KNN-3  & RF   & AB   & MLP     & KNN-1   & KNN-3  & RF    & AB    & MLP   & KNN-1  & KNN-3  & RF    & AB    & MLP   & KNN-1  & KNN-3  & RF    & AB    \\ \hline
\rowcolor[HTML]{CFE2F3} 
Accuracy           & 0.95   & 0.94   & 0.94   & 0.91 & 0.91 & 0.95    & 0.94    & 0.94   & 0.92  & 0.91  & 0.92  & 0.92   & 0.92   & 0.88  & 0.92  & 0.96  & 0.96   & 0.96   & 0.89  & 0.95  \\
Precision          & 0.96   & 0.95   & 0.96   & 0.90 & 0.88 & 0.95    & 0.95    & 0.96   & 0.91  & 0.87  & 0.93  & 0.93   & 0.92   & 0.89  & 0.92  & 1.00  & 1.00   & 1.00   & 0.86  & 0.95  \\
\rowcolor[HTML]{CFE2F3} 
Recall             & 0.94   & 0.92   & 0.92   & 0.93 & 0.94 & 0.96    & 0.92    & 0.92   & 0.93  & 0.94  & 0.92  & 0.90   & 0.91   & 0.88  & 0.92  & 0.93  & 0.93   & 0.93   & 0.91  & 0.95  \\
F1                 & 0.95   & 0.94   & 0.94   & 0.91 & 0.91 & 0.95    & 0.94    & 0.94   & 0.92  & 0.90  & 0.93  & 0.92   & 0.92   & 0.88  & 0.92  & 0.96  & 0.96   & 0.96   & 0.89  & 0.95  \\ \hline
\end{tabular}
}
\end{table*}

\begin{algorithm}
\footnotesize
\caption{Dependency-Aware Individual Construction}\label{algo:sequence_construction}
\begin{algorithmic}[1]
\State \textbf{Input:} A sequence of perturbations $O = [o_1, o_2, \ldots, o_n]$
\State \textbf{Output:} Dependency-aware Sequence $D$
\State $D=[]$

\For{$o \in  O$}
    \State $flag=false$
    \For{$Seq \in D$}
        \For{$o' \in Seq$}
            \If{\Call{HasDependency}{$o', o$}}
                \State Append $o$ to $Seq$
                \State $flag = true$
                \State \textbf{break}
                \EndIf
        \EndFor
        \If{$flag$}
            \State \textbf{break}
        \EndIf
    \If{not $flag$}
        \State Append $[o]$ to $D$
    \EndIf
\EndFor
\EndFor
\State \textbf{return} $D$
% \Procedure{BuildDependencySequence}{$O$}
%     \State Initialize an empty sequence of operation sequences $D$
%     \State $O \gets \text{reverse}(O)$

%     \For{$i \gets 1 \text{ to } \text{length}(O)$}
%         \State Create a new dependency sequence $depSeq \gets [O[i]]$
%         \For{$j \gets i+1 \text{ to } \text{length}(O)$}
%             \If{\Call{HasDependency}{$O[i], O[j]$}}
%                 \State Append $O[j]$ to $depSeq$
%             \EndIf
%         \EndFor
%         \State Append $depSeq$ to $D$
%     \EndFor

%     \State \textbf{return} $D$
% \EndProcedure

% \Function{HasDependency}{$o_i, o_j$}
%     \If{$o_i$.type == `AddNode'}
%         \State $targetNode \gets$ \Call{getOperationInfo}{$o_i$}
%         \State \Return $o_j$.dependsNode($targetNode$)
%     \ElsIf{$o_i$.type == `rewire'}
%         \State $targetNode $, $ $ $targetEdge \gets$ \Call{getOperationInfo}{$o_i$} 
%         \State \Return union($o_j$.dependsNode($targetNode$), $o_j$.dependsEdge($targetEdge$))
%     \ElsIf{$o_i$.type == `remove node'}
%         \State $targetNode \gets$ \Call{getOperationInfo}{$o_i$}
%         \State \Return $o_j$.dependsNode($targetNode$)
%     \ElsIf{$o_i$.type == `add edge'}
%         \State $benignNode $, $endNode \gets$ \Call{getOperationInfo}{$o_i$}
%         \State \Return union($o_j$.dependsNode($benignNode$), $o_j$.dependsNode($endNode$))
%     \EndIf
%     \State \Return \textbf{false}
% \EndFunction
\end{algorithmic}
\end{algorithm}

\subsection{Supplementary on Dependency Determination in Algorithm~\ref{algo:sequence_construction}}

% Algorithm ~\ref{algo:sequence_construction} are used in \S \ref{methodology:individual_representation}.
% This is a supplement on how to determine dependencies in Algorithm ~\ref{algo:sequence_construction}.

Algorithm~\ref{algo:sequence_construction}, which is introduced in Section~\ref{methodology:individual_representation}, is supplemented here with an explanation on how to determine dependencies within the algorithm.
We construct the collection in reverse order of dependencies to determine and return, for each perturbation, whether it has a dependency relationship with the previous operation. Dependency constraints include checking if a deleted node existed previously, if a newly added edge already existed, if a node to be deleted precedes a newly added node, and if a new edge was added before deleting an existing edge. To maintain diversity among genes in individuals, we selectively perform dependency lookup only on key edges and nodes, following specific rules:
\begin{itemize}
    \item For \addnode, check dependencies of its starting node and determine if it's deleted or newly added.
    \item For \rewire, examine the dependencies of the edge and midnode it selects, considering if the edge is newly added and if the starting node is deleted or newly added.
    \item For \deletenode, check dependencies with deleted nodes to identify if they are newly added.
    \item For \addedge, inspect the dependencies of its starting and ending nodes, considering if the nodes are deleted or newly added.
\end{itemize}

\vspace{-0.15cm}
\subsection{Detailed Dataset Information}\label{detailed_dataset}
\vspace{-0.15cm}
\subsubsection{Dataset A}
%一些来自virusshare的恶意样本可能存在标签错误或格式错误，因此我们使用VirusTotal设置为4为一个恶意样本，并且提取它的function call查看里面是否存在恶意的api call，以确保样本的基于FCG的feature是非全0的。
The first dataset includes 6,000 benign samples from AndroZoo~\cite{androzoo} with a VirusTotal~\cite{virustotal} score of 0 and 6,000 malware samples randomly chosen from VirusShare~\cite{virusShare}. 
Some malware samples from VirusShare may have labeling errors or formatting issues. Therefore, we set a threshold of 4 in VirusTotal scores to determine the maliciousness of a sample and extract its FCG. We then check for the presence of malicious API calls to ensure that the FCG-based features are not entirely zero.
The data spans six years from 2018 to 2023, with 2,000 samples collected annually, evenly split between benign and malware categories, resulting in 1,000 samples per category each year. Consequently, there are six sets in total (6×2,000). Each set was divided into 8:2 training and testing sets to ensure that the trained target models achieved excellent performance.
Due to GPU memory limitations of one of the baselines (i.e., HRAT), the dataset size was constrained. 
% \vspace{-15pt}
\subsubsection{Dataset B}
The second dataset is created to evaluate the attack methods, ensuring the malware samples represent various attack vectors. We selected 20 true malware samples from each year between 2018 and 2023, totaling 120 attack samples. These were not included in the training data of the target model, similar to methodologies in other works~\cite{zhao2021structural,li2023black,he2023efficient}. This method guarantees a balanced temporal distribution to avoid bias. Due to semantic integrity requirements~\cite{zhao2021structural, li2023black}, we cannot modify the system functions of samples. Therefore, if essential system functions, which are decision nodes in tree-based models, are absent in the attack samples, the model outputs will not change. This requirement renders over 90\% of our initial attack dataset theoretically unattackable, significantly limiting the effectiveness of tree-based models against adversarial manipulations. Considering these constraints, we specifically selected a new set of 120 theoretically attackable samples for the tree-based models.

\begin{figure}[ht!]
    \centering
    \begin{subfigure}[b]{0.23\textwidth} % 小图宽度
        \includegraphics[width=\textwidth]{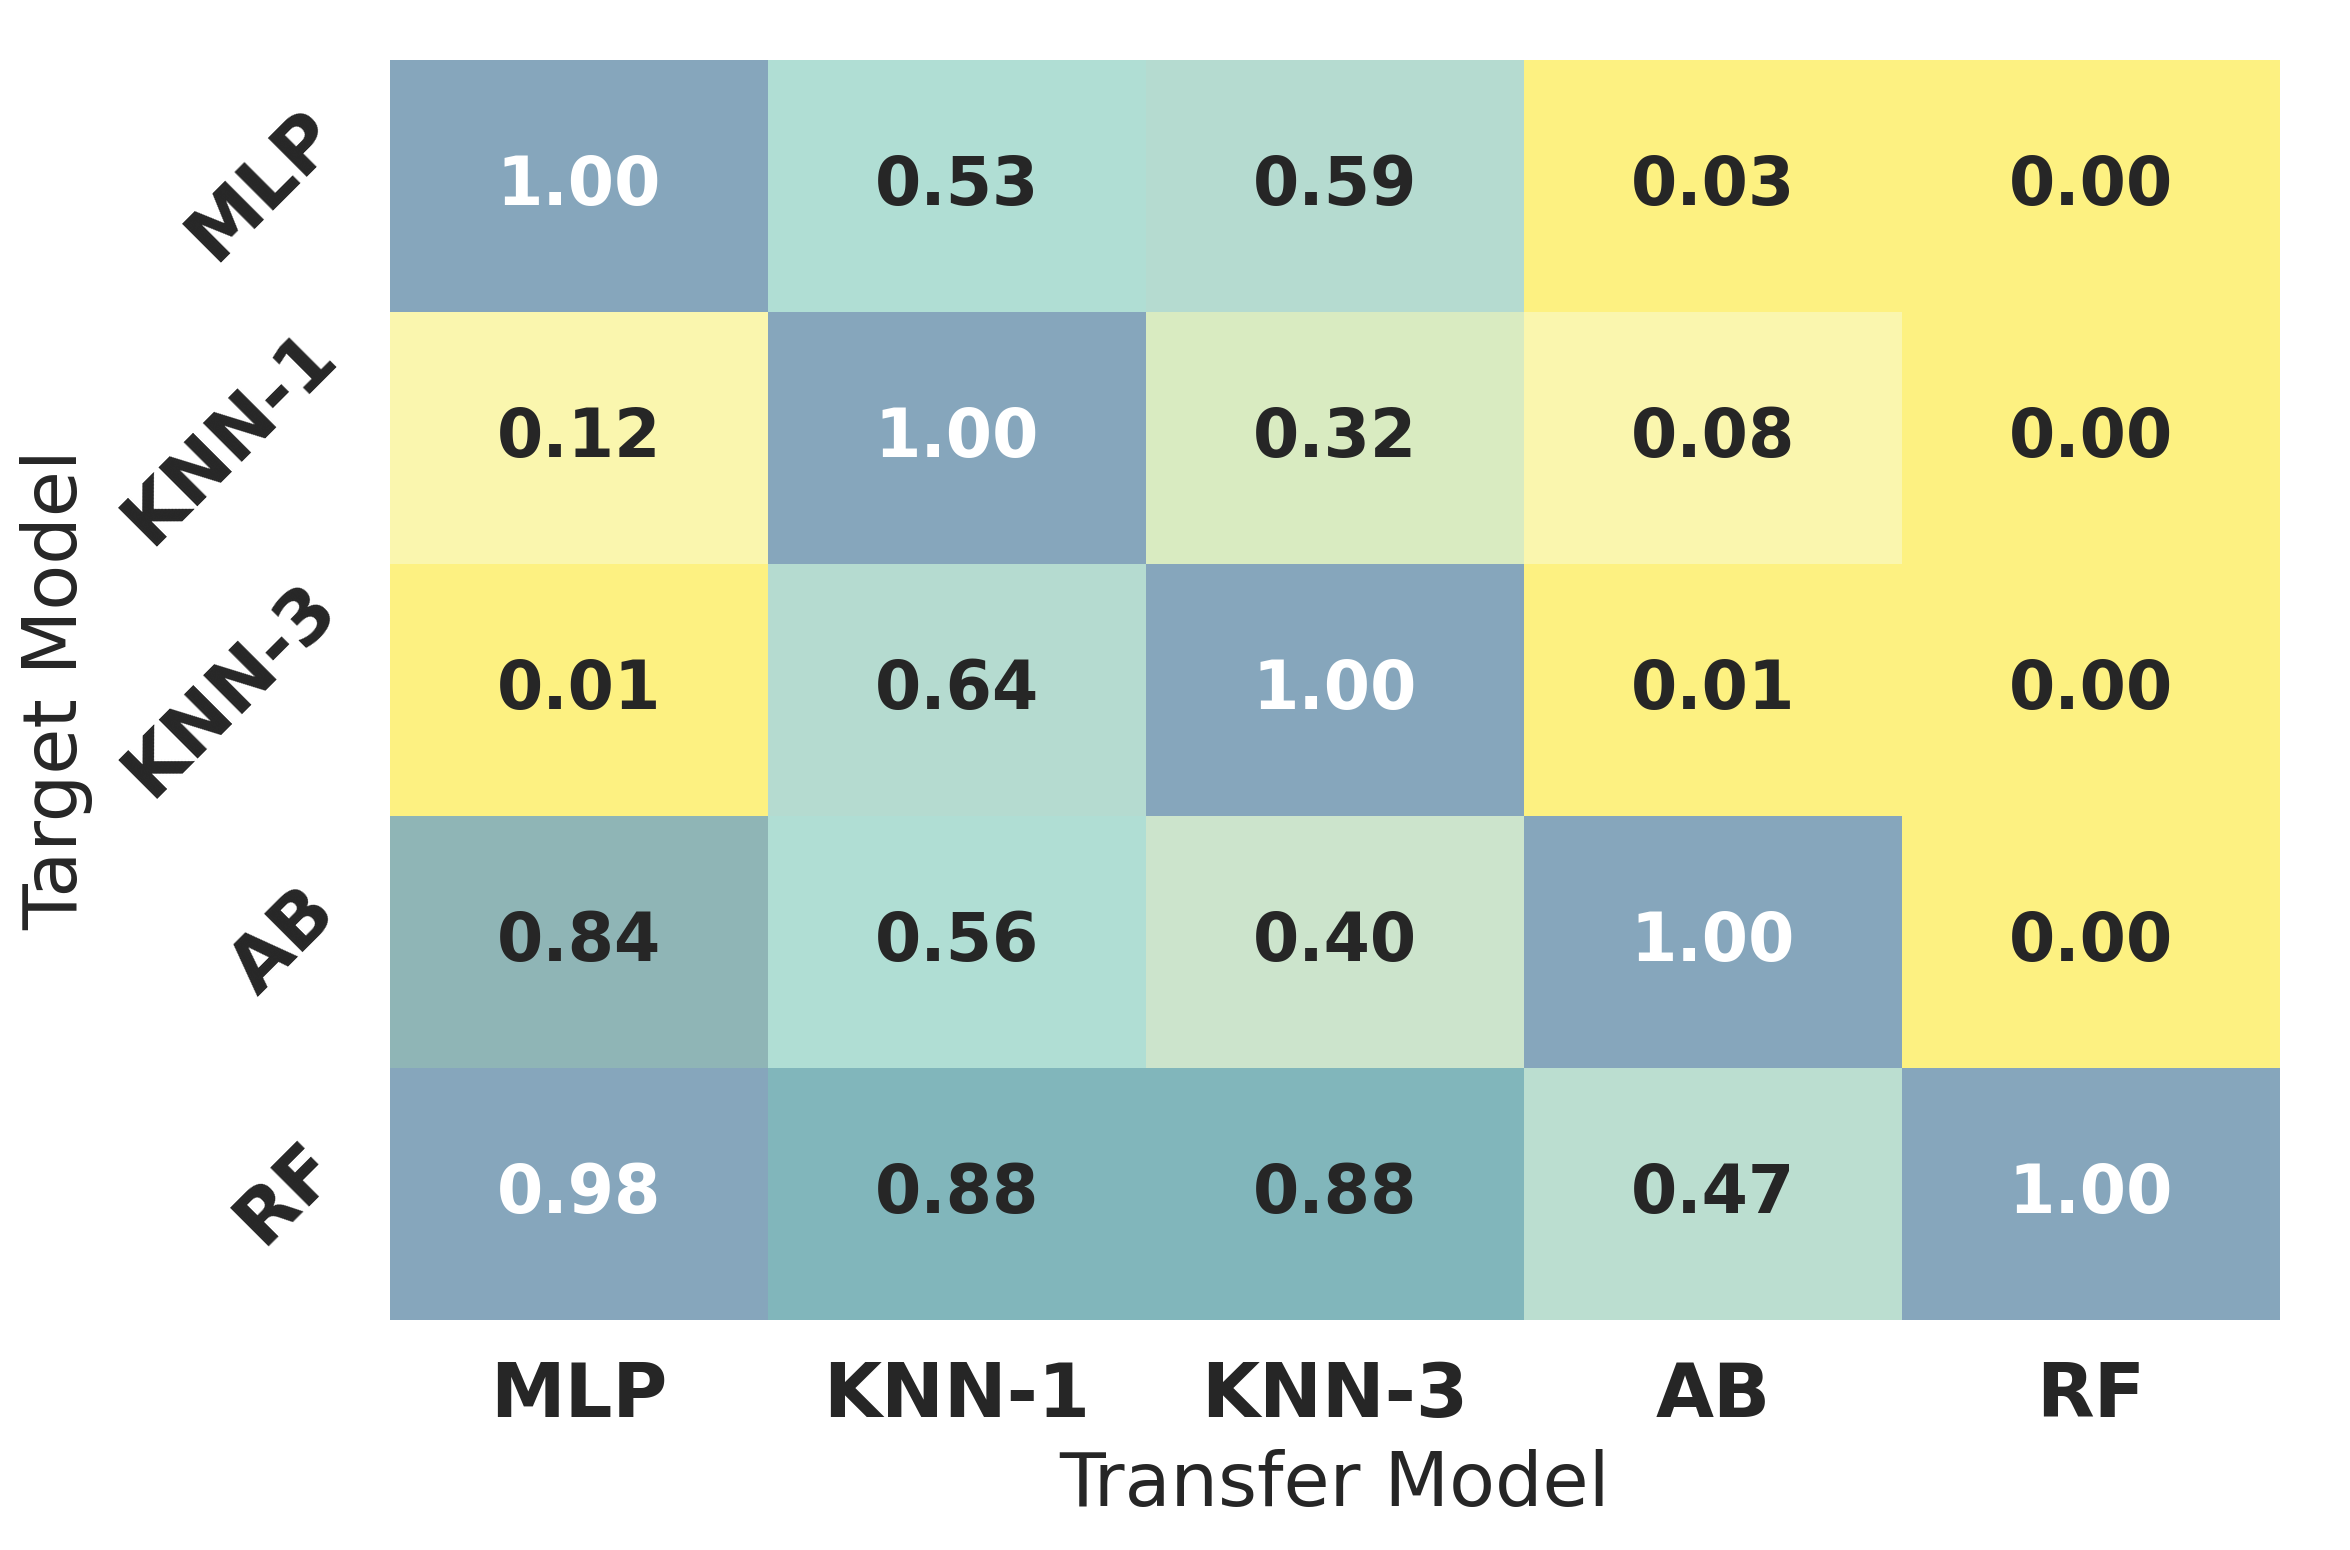}
        \subcaption{MalScan\textsubscript{H}}
        \label{fig:transfer1_malscan_harmonic}
    \end{subfigure}
    \hfill % 用于在小图之间填充空白
    \begin{subfigure}[b]{0.23\textwidth} % 小图宽度
        \includegraphics[width=\textwidth]{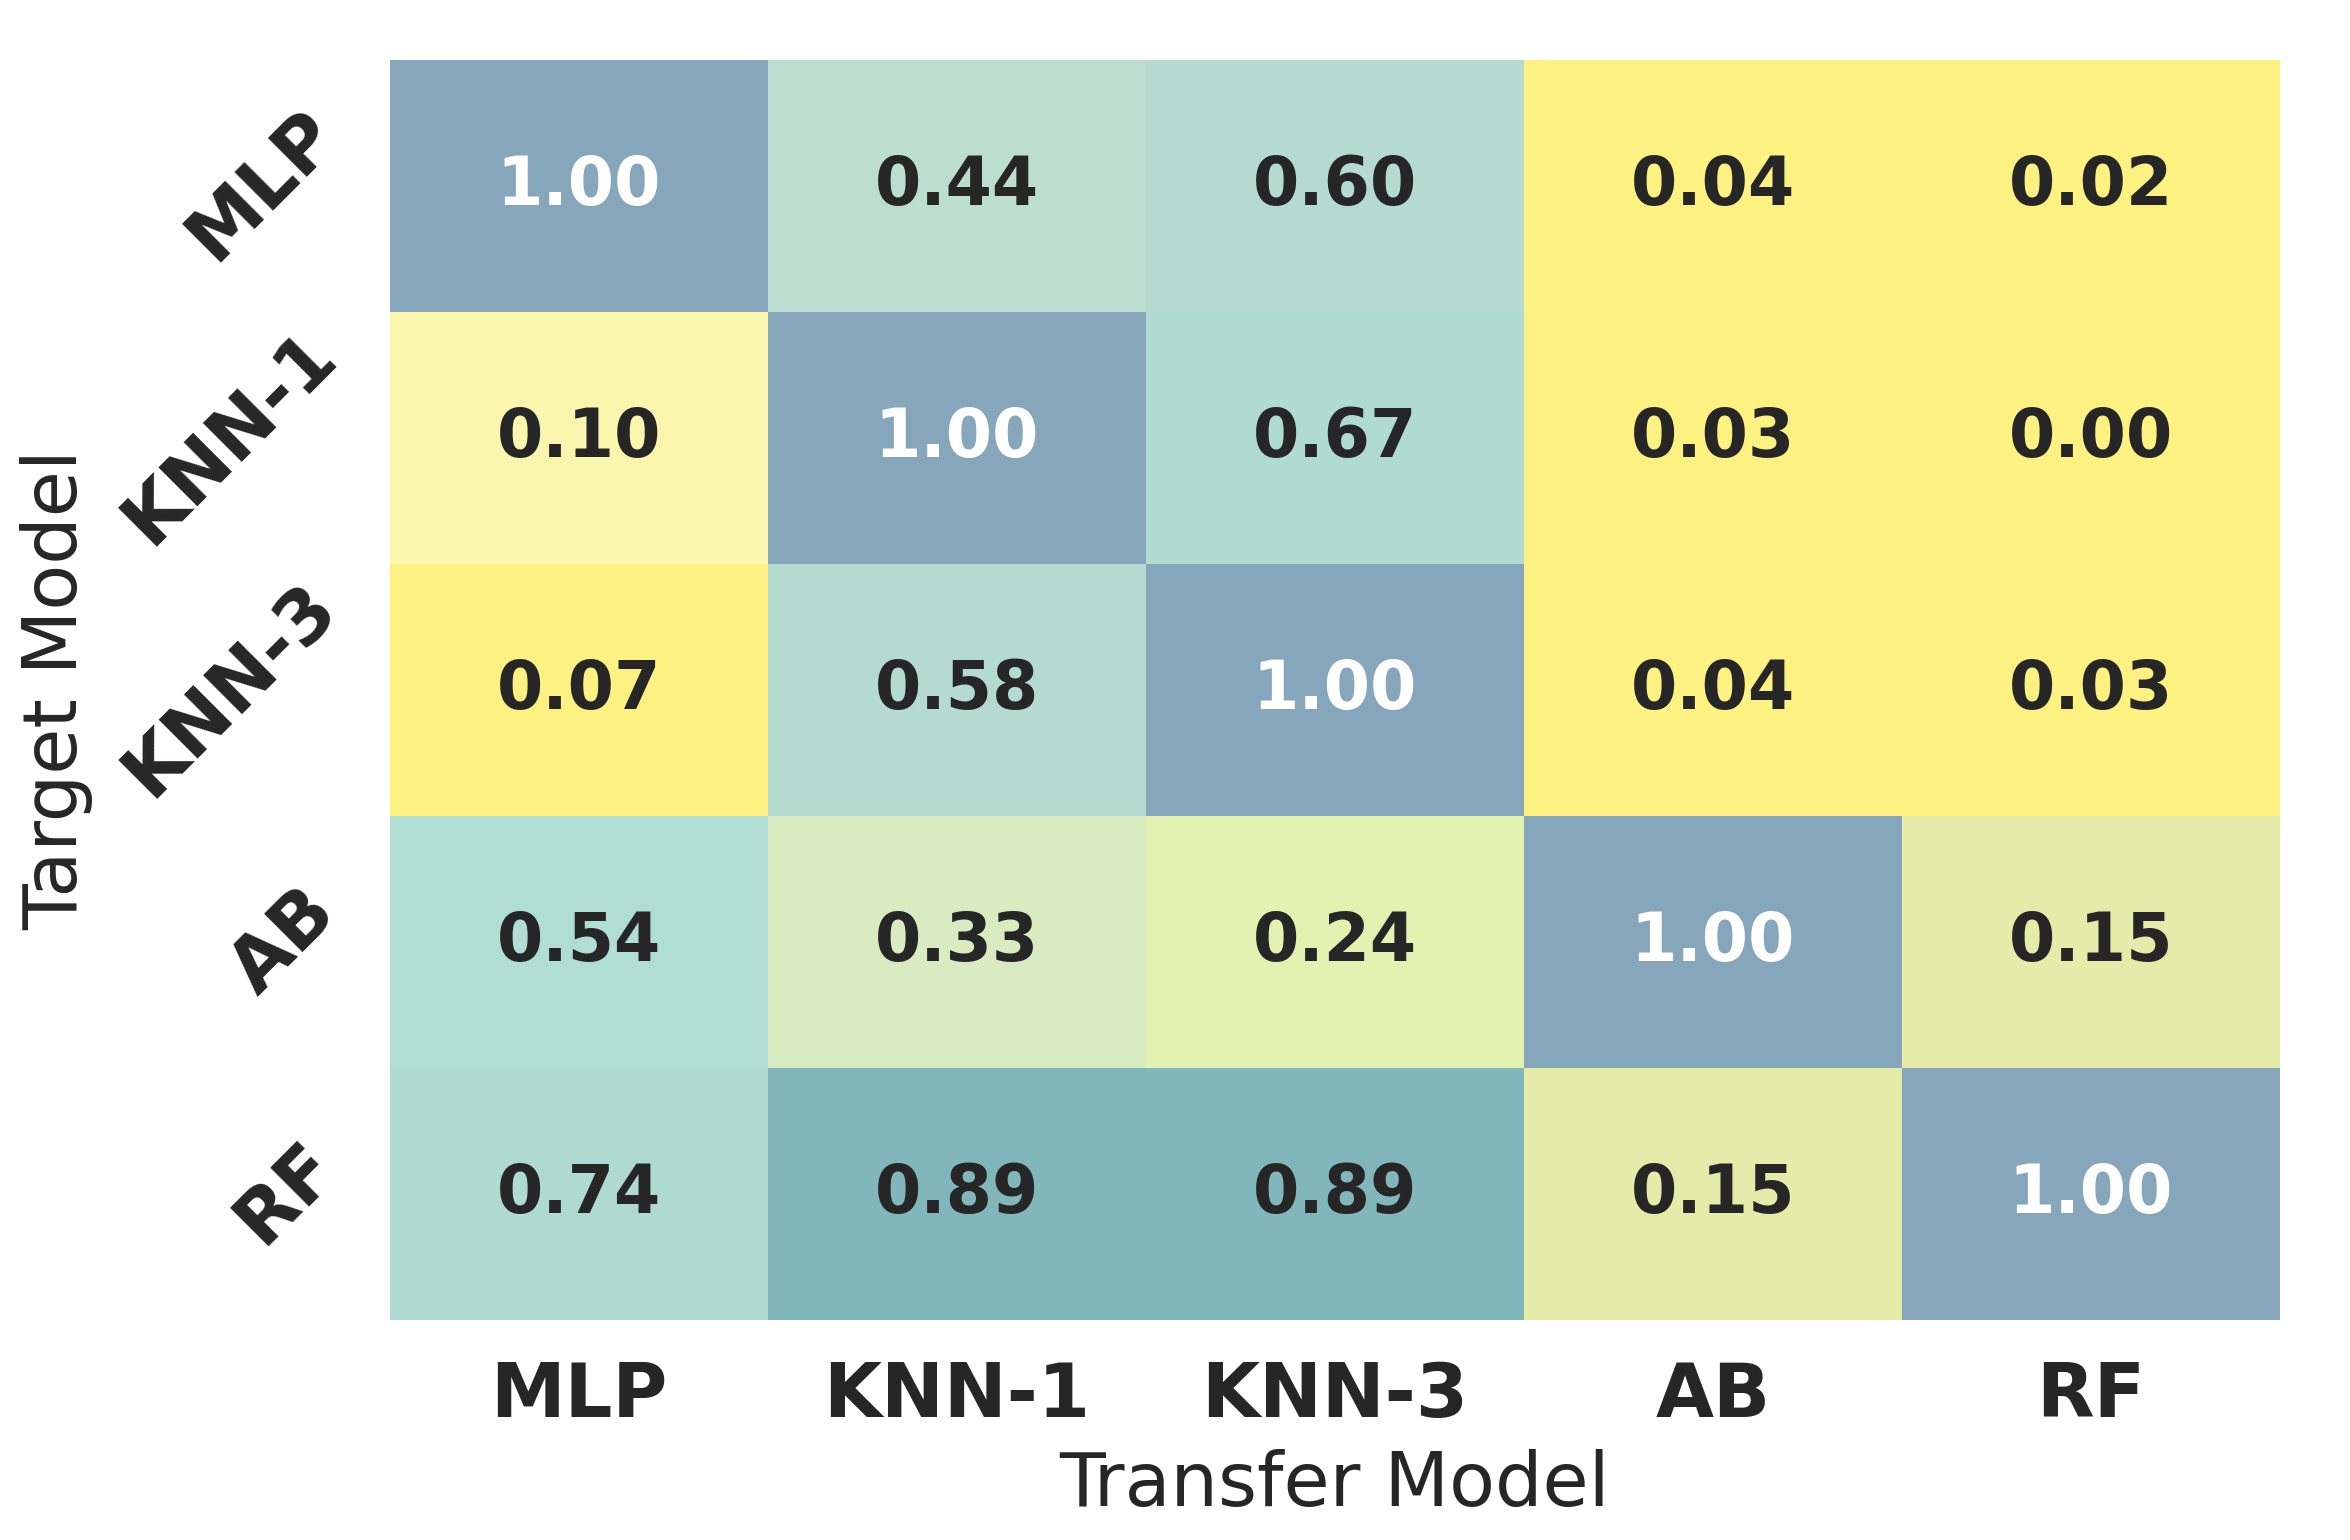}
        \subcaption{MalScan\textsubscript{AVG}}
        \label{fig:transfer1_malscan_avg}
    \end{subfigure}
    % 换行到大图
    \\
    \begin{subfigure}[b]{0.34\textwidth} % 大图宽度
        \includegraphics[width=\textwidth]{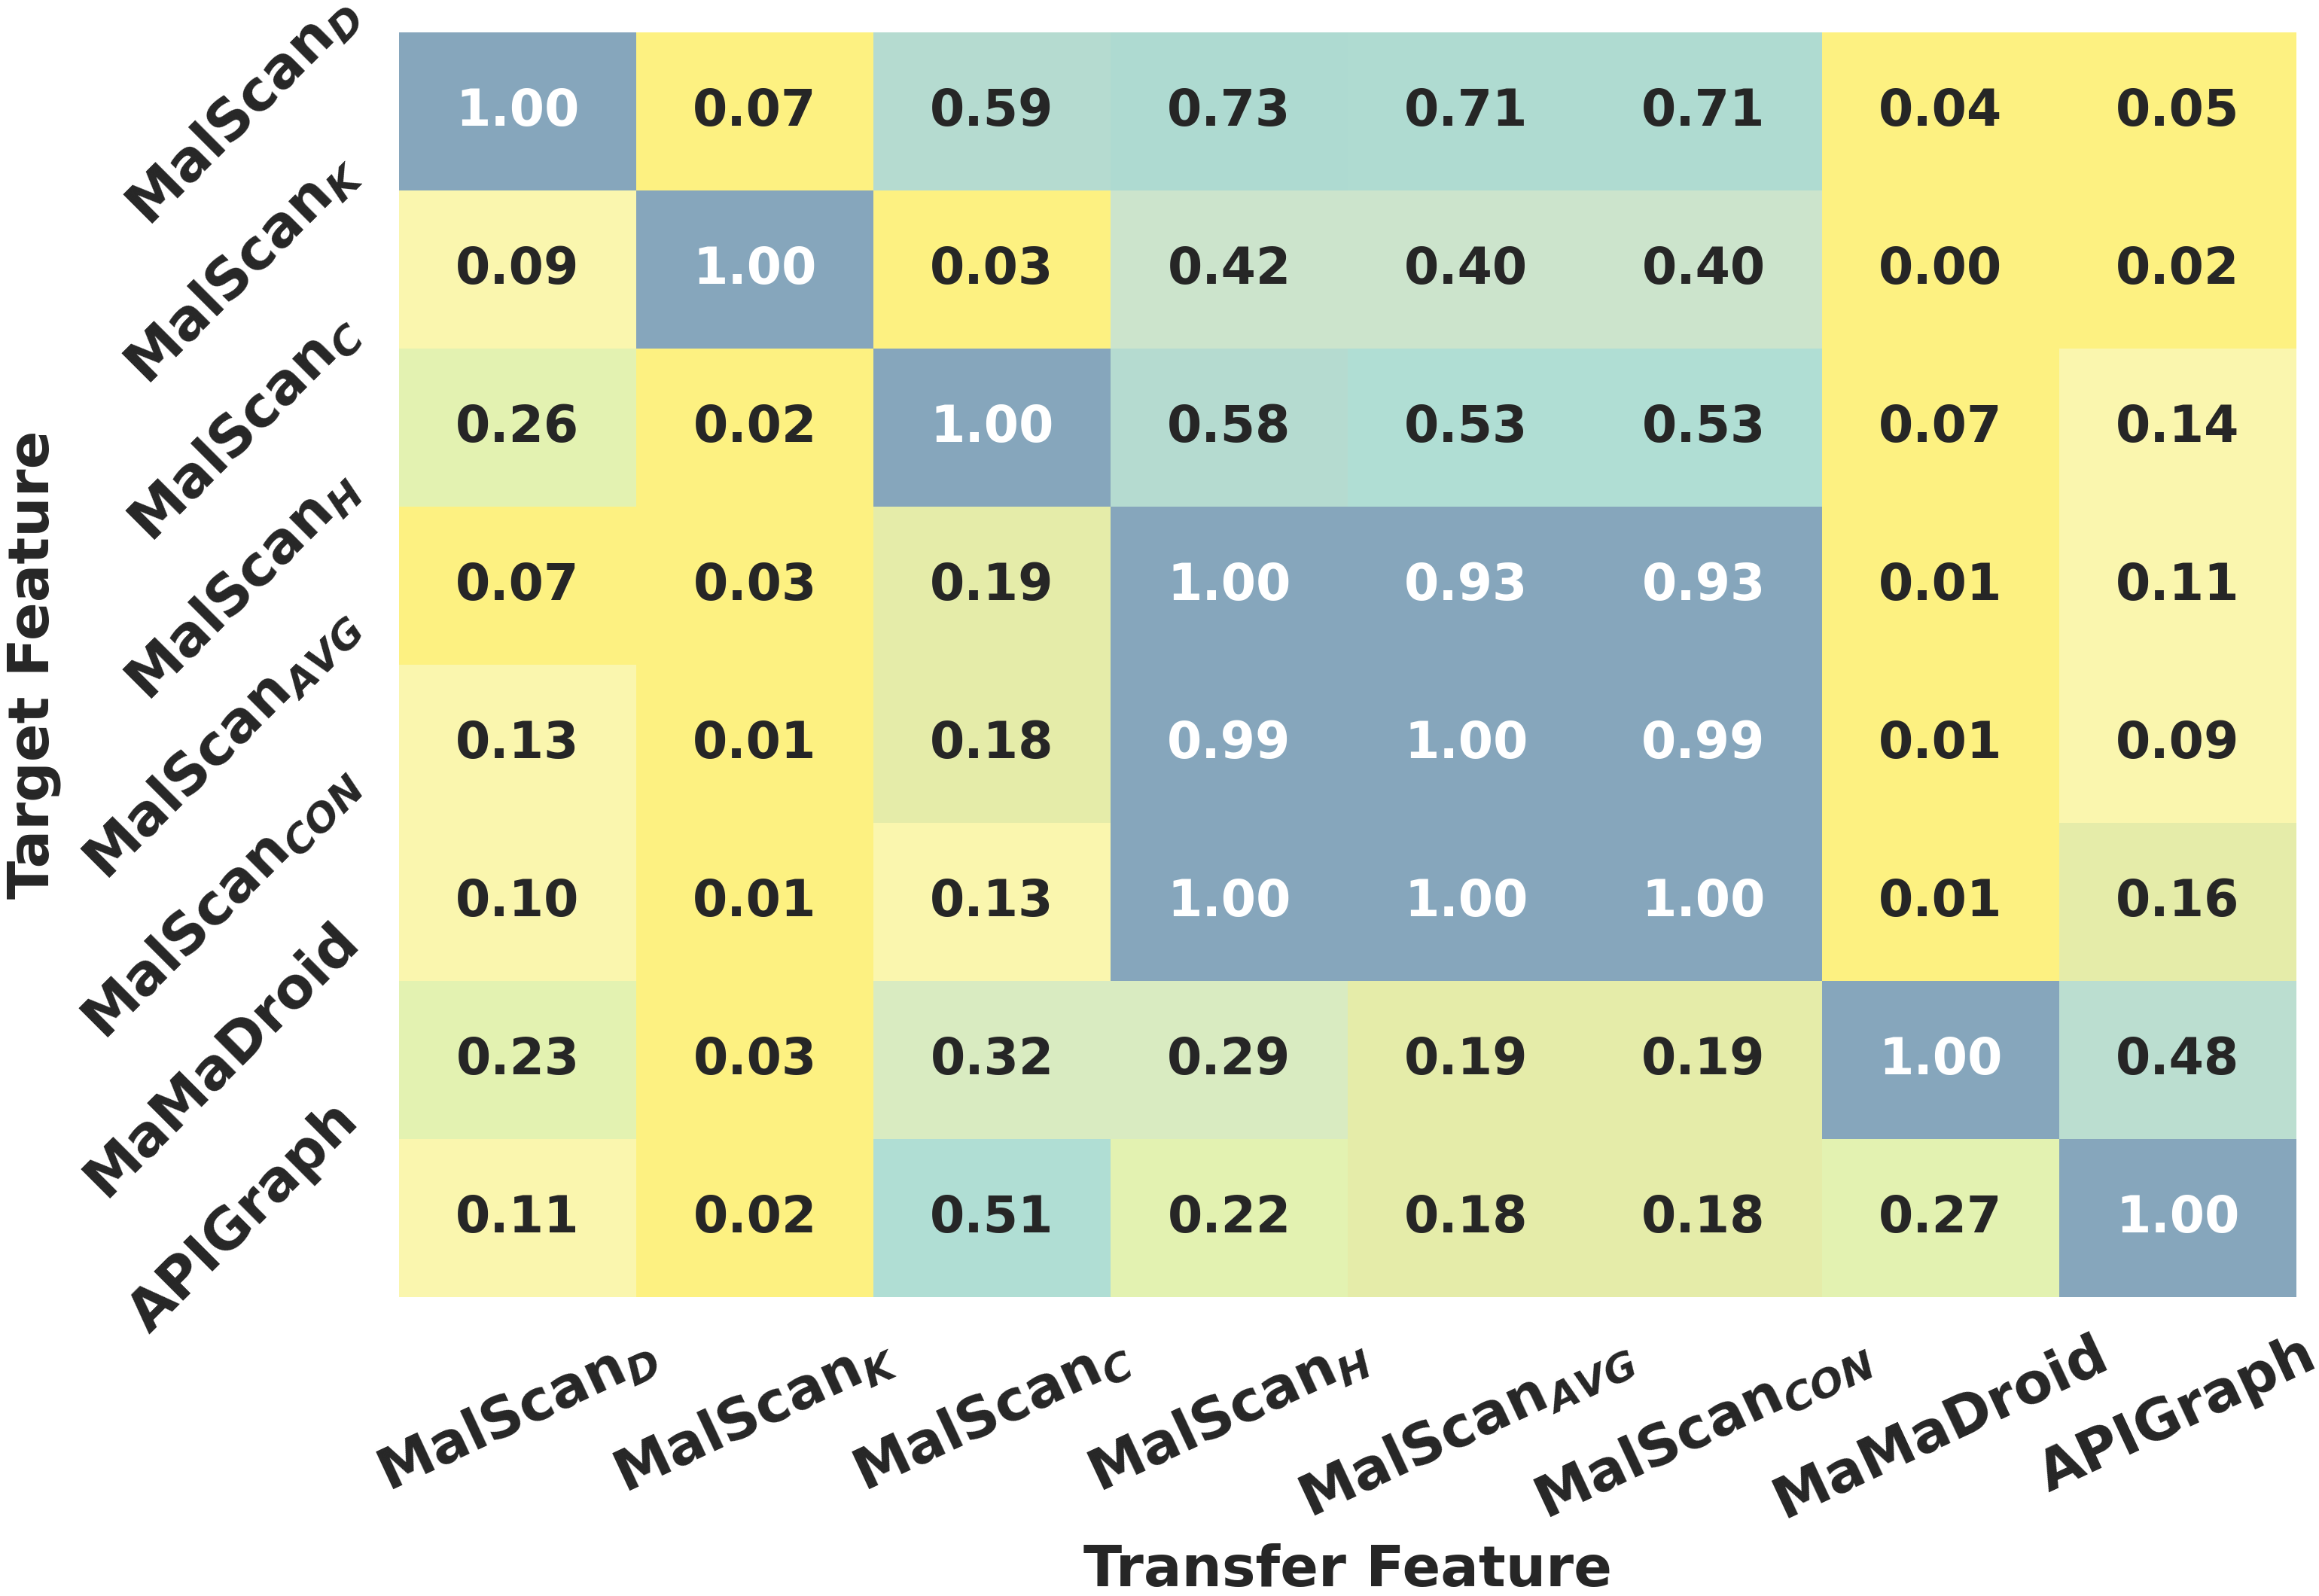}
        \subcaption{KNN-3}
        \label{fig:transfer2_KNN3}
    \end{subfigure}
    \hfill % 用于在大图之间填充空白
    \begin{subfigure}[b]{0.34\textwidth} % 大图宽度
        \includegraphics[width=\textwidth]{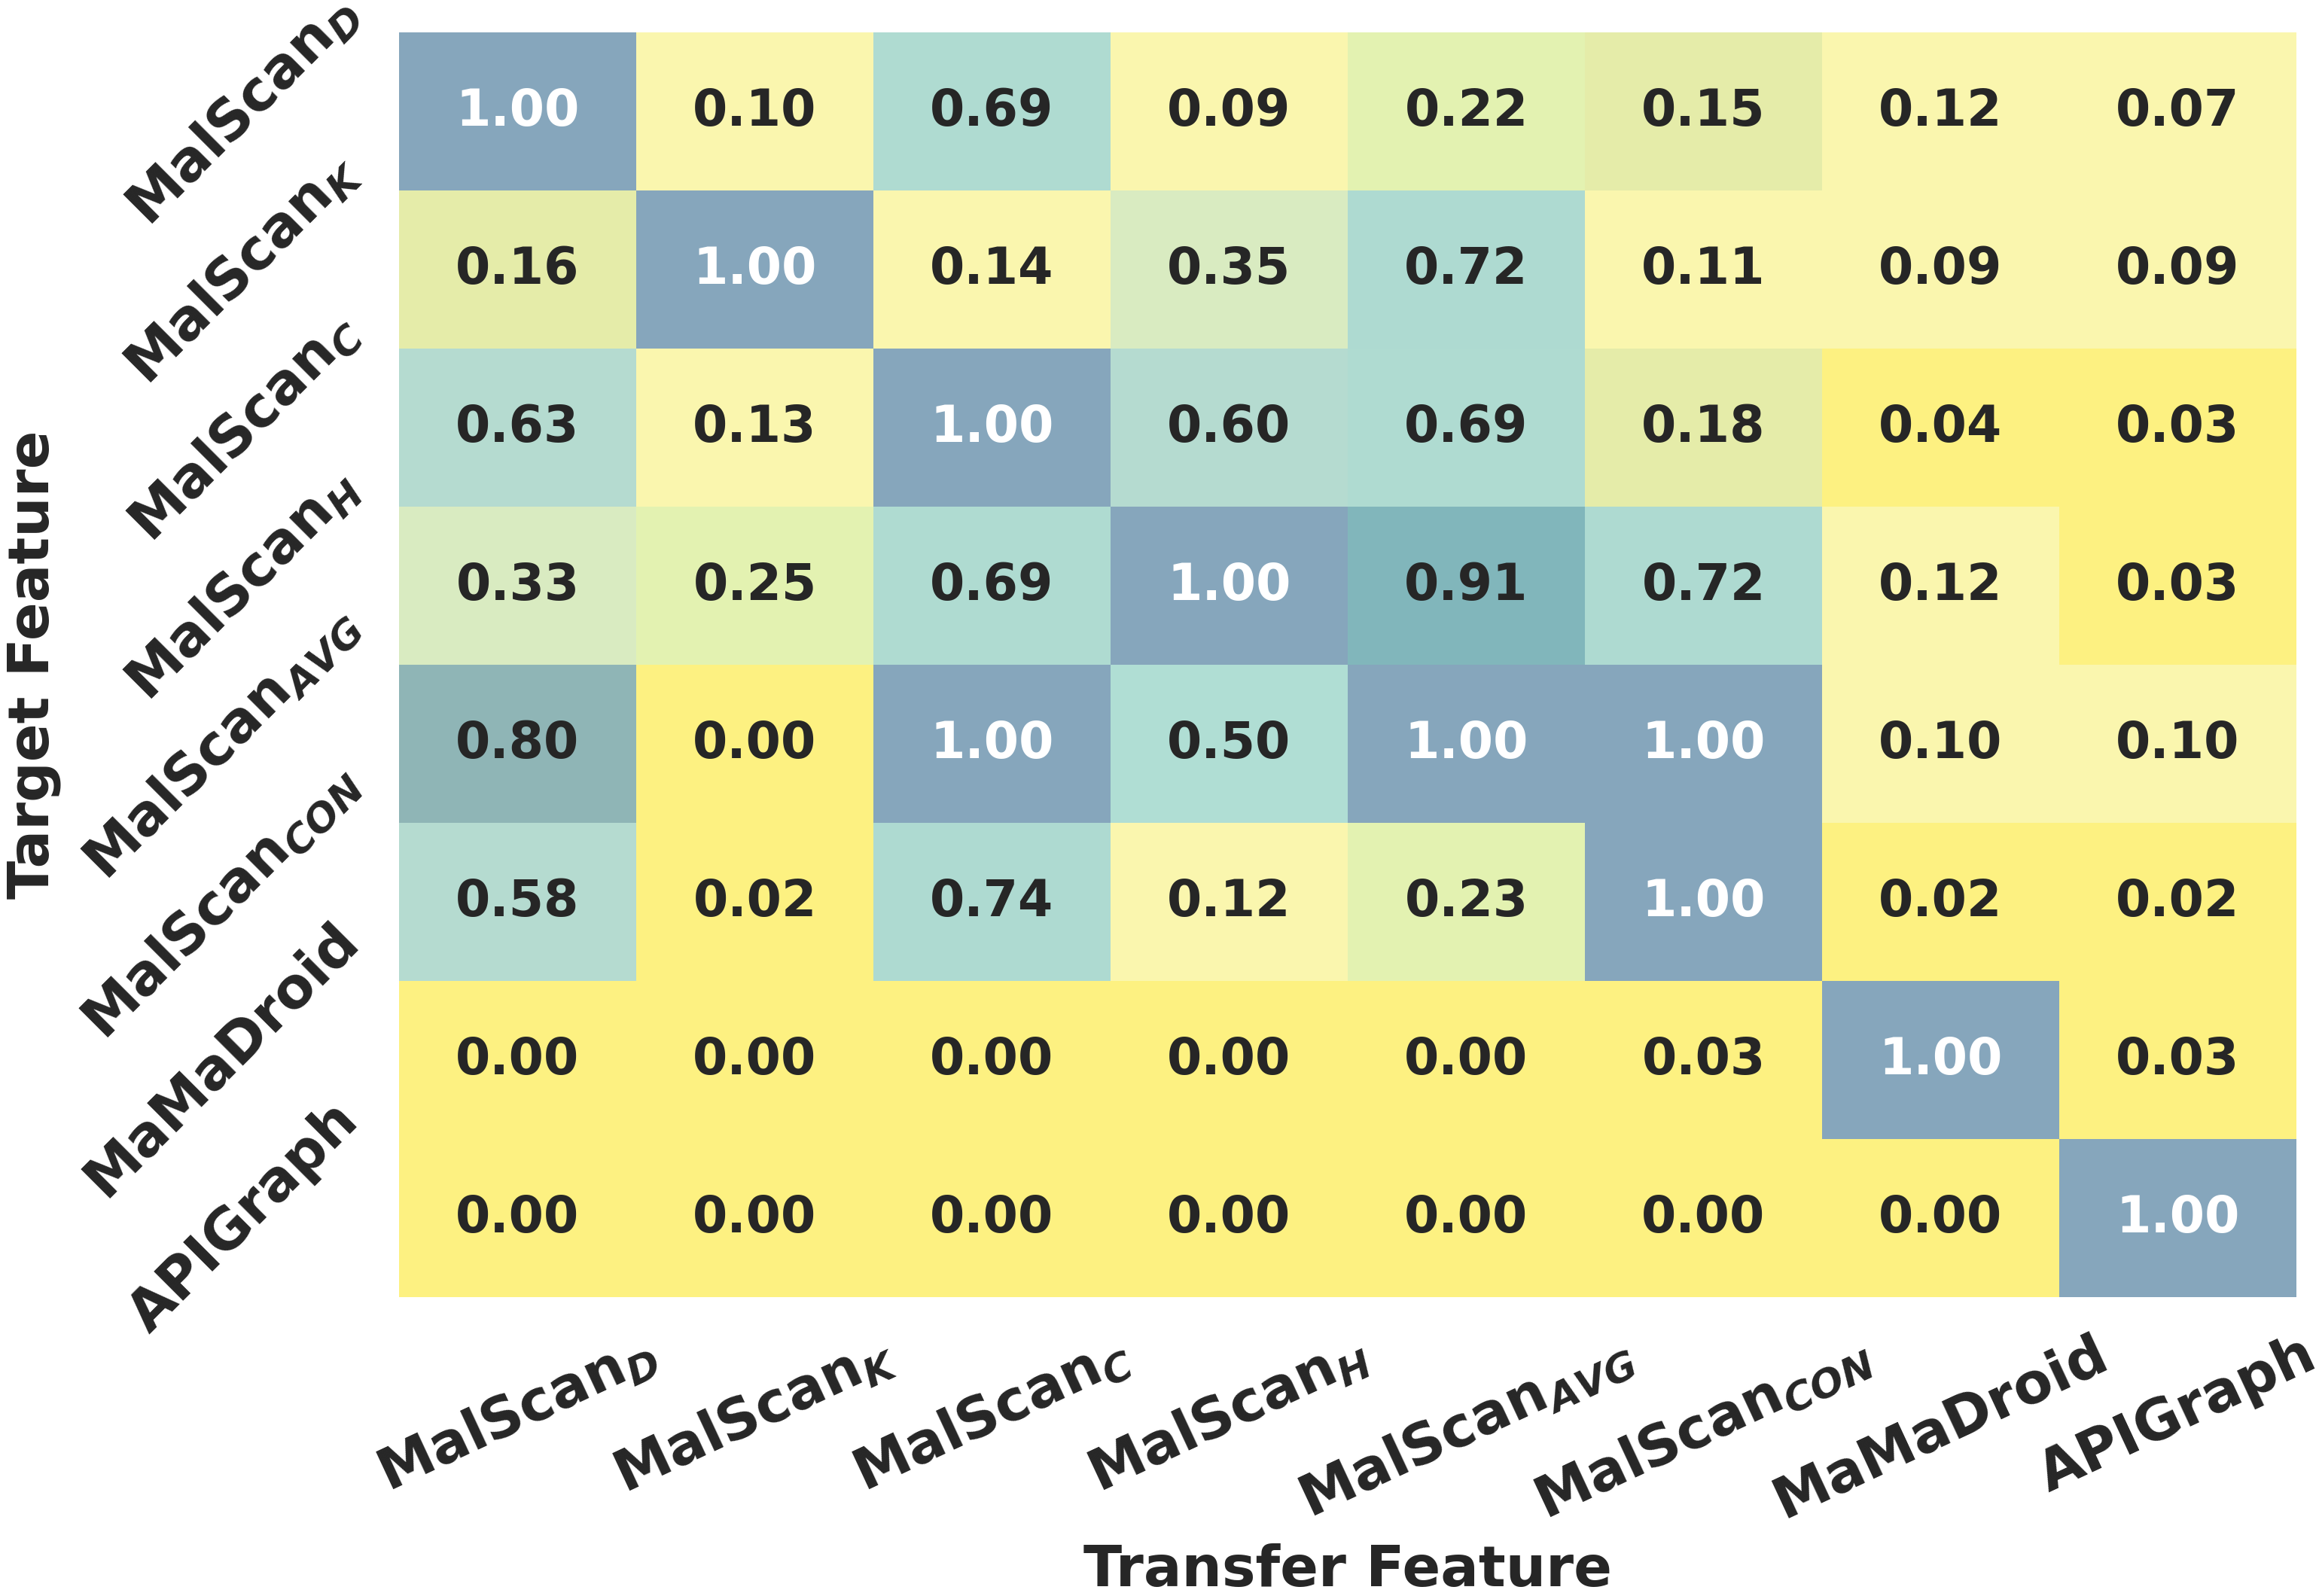}
        \subcaption{AdaBoost}
        \label{fig:transfer2_AB}
    \end{subfigure}
    
    \caption{Transferability in between different features and models (Supplementary for Figure~\ref{fig:transfer} in \S \ref{evaluation:RQ4 adaptability})}
    \label{fig:transfer_appendix}
    \vspace{-15pt}
\end{figure}
\vspace{-0.15cm}
\subsection{Discussion on Baselines}\label{resonforwhy}
\vspace{-0.15cm}
\subsubsection{Challenges in \hrat's Replicability}
In our evaluation~\ref{evaluation:RQ1 effectiveness}, the performance of \hrat differed significantly from the claims made in the paper, prompting us to conduct a detailed analysis.
Indeed, its replicability was also proven challenging in another survey article~\cite{olszewski2023get}.

% The \hrat~\cite{zhao2021structural} is the first to propose using graph structures as the target of attack, indirectly guiding classifiers to make incorrect decisions through perturbations in the problem space, presenting an innovative approach to adversarial attacks.
In \hrat~\cite{zhao2021structural}, the process of conducting adversarial attacks on graph structures is defined as a reinforcement learning process. Specifically, the researchers have defined four types of graph modification rules that maintain semantic consistency. Utilizing a DQN, these four operations are considered as potential actions to determine which one to execute. In each action, given that the graph can be represented as an adjacency matrix, a gradient calculation is performed across the entire graph to select the position with the highest gradient for the operation. If the operation successfully reverses the sample's label, a positive reward is obtained; otherwise, a negative reward is received, the magnitude of which correlates with the changes in the number of edges and nodes in the graph.

As illustrated in Table 1, they mainly focus on a subset of graph embedding methods from \malscan, \mamadroid, and \apigraph, while the downstream classifier of choice is confined to KNN with \( k = 1 \). Given KNN's reliance on instance-based learning, it necessitates the loading of the entire training set into memory. This requirement becomes problematic when gradient-dependent computations are executed, particularly if these calculations are to be GPU-accelerated. The inevitable result is the exhaustive consumption of GPU memory by the KNN model's training set, a concern exacerbated by the annual increase in the size of Android APKs.
Additionally, integrated classifiers such as AdaBoost and Random Forest are non-differentiable, rendering the gradient search technique, as utilized by the authors, ineffective. It is also claimed that since the attacks perturb graph structures and not feature vectors, the feature extraction methodology does not influence the attack process. However, in reality, feature extraction methods vary significantly and have unique vulnerabilities. Basic reinforcement learning, lacking a highly targeted reward system, cannot guarantee effectiveness across all feature extraction methods.
Particularly, \malscan and \mamadroid employ distinct feature extraction methodologies, with \malscan being sensitive to both node and edge alterations, whereas \mamadroid is primarily affected by edge additions, with node changes having minimal impact. Furthermore, some feature extraction methods have high computational demands, like the closeness metric in \malscan, which requires the calculation of shortest paths from a node to all other nodes in the graph—this demands substantial memory and computational time.
Most critically, despite gradient-based attack methodologies proving effective in early adversarial scenarios, the gradient search approach employed in the paper for estimating perturbation locations is rudimentary and imprecise. Altering a zero to a one in the adjacency matrix of a graph is a significant change, not as nuanced as adjusting from zero to 0.01. Our experiments reveal the inefficiency of the methods, both in terms of attack success rates and computational overhead, contradicting their claims of perfection.
%(e.g., achieving over 90\% success rate in all scenarios).

\subsubsection{Reproduction of \bagammo}
%我们使用了一个5层的GCN对bagammo的复现，结构如下。
We replicated \bagammo using a five-layer GCN, which is designed to process edge data along with node in-degrees and out-degrees as input features. The network architecture progressively increases feature dimensions from 16 to 128 across its layers, incorporating ReLU activations and dropout after each layer to prevent overfitting. The training was conducted on a GPU, utilizing a DataLoader with shuffled batches and the Adam optimizer with a learning rate of 0.001, across 100 epochs. We employed CrossEntropyLoss to evaluate performance metrics. Each training epoch included a sequence of forward propagation, loss assessment, backpropagation, and parameter updates. Upon completion of the training, the model achieved an accuracy of approximately 80\%.

\begin{figure}
  \centering
\includegraphics[width=0.43\textwidth]{ICSE25/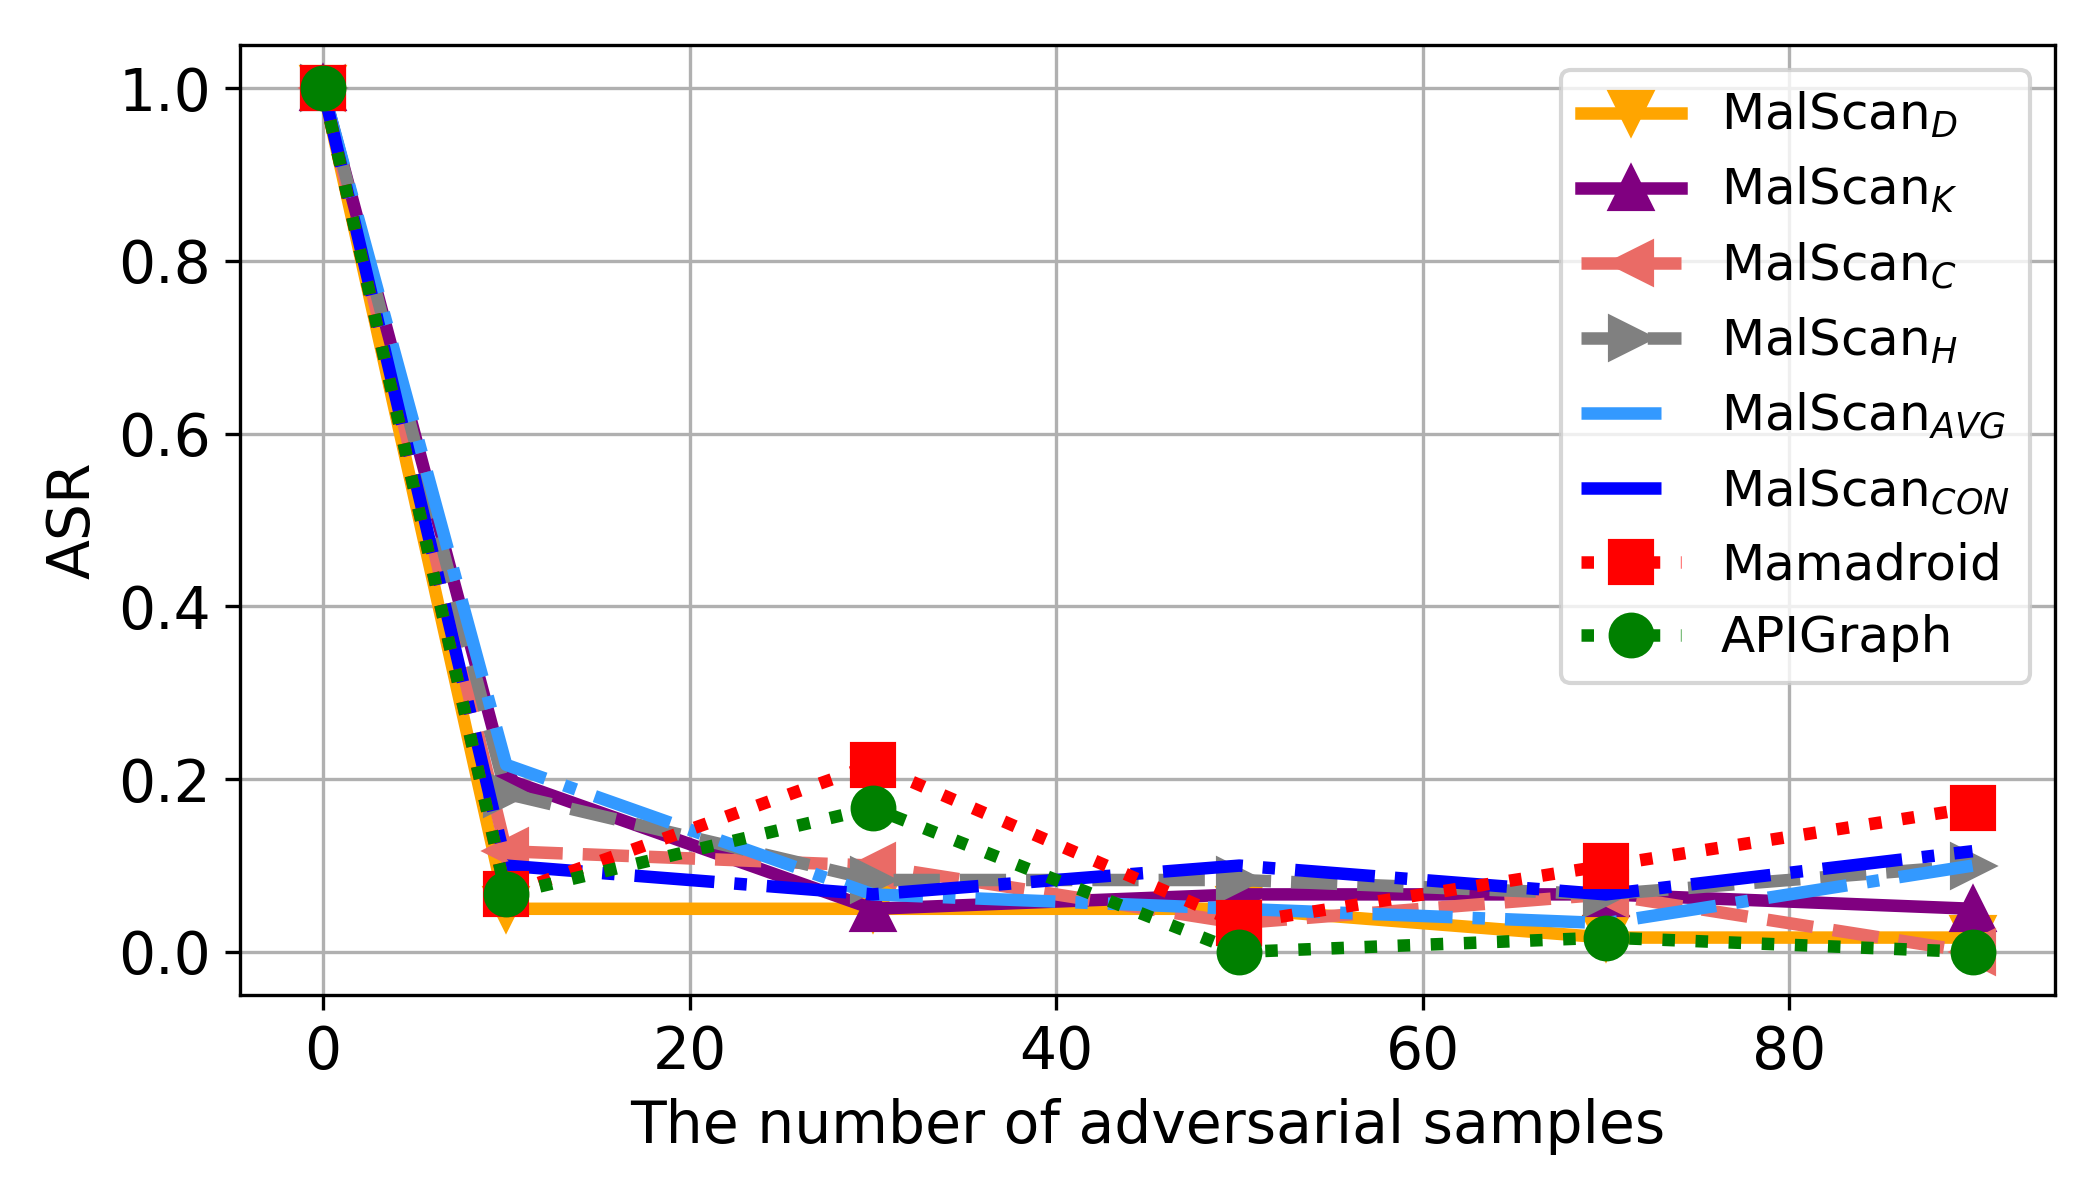}
  \caption{Attack success rate after retraining}
  \label{fig:retrain}
\end{figure}

\subsection{Supplementary for Transferability Analysis}
Due to space limitations, some experimental results of transferability analysis in \S \ref{evaluation:RQ4 part1} are presented in Figure~\ref{fig:transfer_appendix} of Appendix. Since the results of MalScan\textsubscript{H} are similar to those of MalScan\textsubscript{C}, and MalScan\textsubscript{AVG} is akin to MalScan\textsubscript{CON}, we put the results for MMalScan\textsubscript{H} and MalScan\textsubscript{AVG} in Figure~\ref{fig:transfer_appendix} (a-b) of the Appendix. From the perspective of classifiers, the results of KNN-3 are similar to those of KNN-1. Although AdaBoost results differ from those of Random Forest, the latter is more representative. Therefore, the results for KNN-3 and AdaBoost are also included in Figure~\ref{fig:transfer_appendix} (c-d) of the Appendix.

\subsection{Enhancing ML Models Robustness through 
Adversarial Retraining}\label{retrain}
We further explored the impact of adversarial samples generated by \tool on enhancing model robustness. Specifically, we enhanced the original training set (i.e., Dataset A in \S \ref{evaluation:setup}) with 90 adversarial samples and tested the improved model's resilience using an independent set of 60 adversarial samples, aiming to verify the mitigation of previously identified vulnerabilities. During the retraining process, we varied the number of adversarial samples in the training set from 10 to 90 to observe changes in the ASR from the test samples. 

As shown in Figure.~\ref{fig:retrain}, as adversarial samples are introduced into the training set, there is a sharp decline in ASR for all features. This decrease is most pronounced within the first 10 samples added, indicating that retraining with even a small number of adversarial samples significantly enhances model robustness.
However, different features show different levels of resilience. For example, features like \mamadroid show higher or more erratic ASR values even with increased adversarial training, which may indicate the model is susceptible to overfitting and forgetting previously correct patterns due to \mamadroid's family features being quite low-dimensional (i.e., 121 dimensions). 
Similarly, the issue also appears in \apigraph, although it is less severe than in \mamadroid.
In contrast, features like \malscan might be more stable because they capture a broad and complex set of behaviors or characteristics, making them less prone to drastic shifts in performance with the introduction of adversarial examples.
Thus, during retraining, it is crucial to choose a suitable ratio of adversarial samples for different feature types to mitigate this issue.  In summary, the adversarial examples generated by \tool could be effectively used to enhance the resilience of ML-based models.
